# Supplementary material for: Can we trust LLMs as a tutor for our students? Evaluating the Quality of LLM-generated Feedback in Statistics Exams
Source: arXiv:2511.04213 source file (2025-11-06)
Supplement: Supplementary file 1 [file supplementary-exam-translated.pdf]

## Task 1

Tick the correct answer(s) for each question:

a) Tick all measures of central tendency. (*knowledge; central tendency*)
   (a) Arithmetic mean
   (b) Median
   (c) Standard deviation
   (d) Mode

b) Which statement is correct? (*knowledge; dispersion*)
   (a) The variance is the average absolute amount of the deviation from the arithmetic mean.
   (b) The variance is the average quadratic deviation from the arithmetic mean.

c) Which measures of association are suitable for nominal variables? (*knowledge; correlation*)
   (a) Rank correlation and correlation coefficient
   (b) Coefficient of contingency

d) Tick the correct statements. (*knowledge; visualization*)
   (a) The terms Histogram and Bar plot are interchangeable.
   (b) Histograms are suitable for displaying frequency distributions of metric characteristics.
   (c) In histograms, the areas represent the (relative or absolute) class frequencies.

e) You want to examine the relationship between a variable indicating whether someone receives tutoring and a variable indicating whether someone passes the exam. Which measure of association is appropriate? (*knowledge; correlation*)
   (a) Spearman rank correlation
   (b) Pearson correlation coefficient
   (c) Odds Ratio
   (d) Variance

f) Choose the correct answers regarding the intercept in regression analysis. (*knowledge; regression*)
   (a) The intercept always crosses the point (x = 0, y = 0).
   (b) Intercept and axis section mean the same thing in regression analysis.
   (c) The intercept is the value y takes, when x = 0.

g) The residual is: (*knowledge; regression*)
   (a) The difference between the observed value for y and the predicted value for y.
   (b) The difference between the observed value for x and the predicted value for x.
   (c) The square of the correlation coefficient.

h) Which measures are not robust? (*knowledge; central tendency*)
   (a) Arithmetic mean
   (b) Median
   (c) Variance
   (d) Standard deviation

## Task 2

a) Ear length of rabbits are shown both as a histogram and a boxplot. Which information (especially central tendency) can you determine more easily from the boxplot, and which from the histogram? (*interpretation; visualization*)

b) Is the mode or median larger for this variable? (*interpretation; central tendency*)

c) Is the statement "A rabbit with an ear length of 7 cm lies within the middle 50% of the observations" correct? (*interpretation; visualization*)

d) The arithmetic mean is not directly visible from either plot. Do you estimate it to be larger or smaller than the median? Justify briefly. (*interpretation; visualization*)

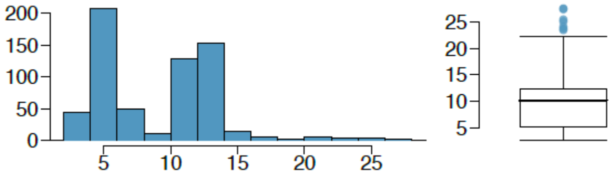


Figure 1: Graph for task 2a

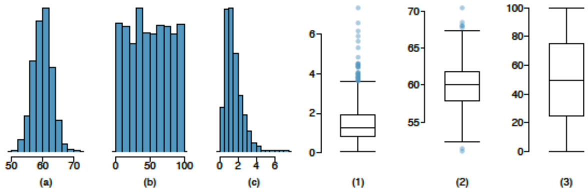


Figure 2: Graph for task 2e

e) *For students not in Media Informatics* Match each boxplot with the histogram showing the same variable. (*interpretation; visualization*)

f) *For Media Informatics students* You have a dataset `osterhasen` containing ear length (`length`) and color (`color`) of rabbits. You already received an R-code, with which you can generate a histogram of the ear length: `ggplot(osterhasen, aes(x = length)) + geom_histogram`. How do you need to adjust the code to receive boxplots with the ear length separated for the colors of rabbits? (*R; R*)

## Task 3

According to a survey conducted by DAK-Gesundheit in 2022, at the time of the survey, around 23 percent of respondents believed that fasting was very beneficial to health, while around 41 percent of participants said that fasting was beneficial to health. About 20 percent said that they found fasting less beneficial to health. 13 percent of those surveyed were of the opinion that fasting was not beneficial to health at all.

a) What is the scale level of this variable? (*calculation; variables*)

b) Can the mode be determined meaningfully? If yes, state it. (*calculation; central tendency*)

c) Can the median be determined meaningfully? If yes, state it. (*calculation; central tendency*)

d) Can the arithmetic mean be determined meaningfully? If yes, state it. (*calculation; central tendency*)

e) The Easter Bunny Foundation commissions a new study on the advertising budget of confectionery manufacturers. You see the results in figure 3. You are tasked with summarizing the distribution of advertising budgets in a single measure. Which one do you choose? Explain your choice in no more than two sentences and indicate the value of the chosen measure. (*calculation; central tendency*)

f) Provide the 25% and 75% quantiles. (*knowledge; central tendency*)

## Task 4

A farmer sells brown (b) and white (w) eggs. A customer claims white eggs have less variation in weight. He tries to investigate that with the data in figure 4.

a) Calculate and compare the variances and standard deviations for white and brown eggs. (*calculation; dispersion*)

b) *For non-Media Informatics students* Determine the interquartile range for all eggs combined. (*calculation; dispersion*)

c) *For Media Informatics students* Given an R dataset `eier` with variable `gewicht`, write R code to calculate the standard deviation. (*R; R*)

| Unternehmen | Werbebudget Mio. EUR |
|---|---|
| Storck und Hase | 82 |
| Hasenfoods | 52 |
| Ritter Hase | 29 |
| Kraftgras Foods | 27 |
| Osterrero | 233 |
| Hasibo | 27 |
| Hoppley | 37 |
| Mümmelsen | 16 |
| Lindt & Springli | 25 |

Figure 3: Graph for task 3e

| Ei | Farbe | Gewicht in g |
|---|---|---|
| 1 | b | 54 |
| 2 | w | 49 |
| 3 | b | 72 |
| 4 | w | 58 |
| 5 | b | 61 |
| 6 | b | 60 |
| 7 | w | 31 |
| 8 | w | 66 |

Figure 4: Graph for task 4

## Task 5

For the days before and after eastern, following data on consumption of Easter eggs in a southern-german city are available:

a) Calculate the Pearson correlation coefficient $\rho(X,Y)$ and interpret it. (*calculation; correlation*)

b) Would changing the X-variable from "days before/after Easter" to actual dates change the correlation coefficient? Explain briefly. (*interpretation; correlation*)

c) A consultant wants to decide whether to increase or decrease production in May. What conclusions can you draw from the correlation coefficient? Explain briefly. (*interpretation; correlation*)

## Task 6

The following contingency table shows pet ownership by gender.

a) Complete the table with marginal totals. (*calculation; frequencies*)

b) Calculate the $\chi^2$ coefficient. (*calculation; correlation*)

| Zeit vor/nach Ostern (X, in *Tagen*) | Konsumierte Ostereier (Y, in $t$) |
|---|---|
| -2 | 0 |
| -1 | 3.7 |
| 0 | 9.0 |
| 1 | 6.2 |
| 2 | 3.2 |

Das Osterküken erstellt aus den Daten die folgende Grafik

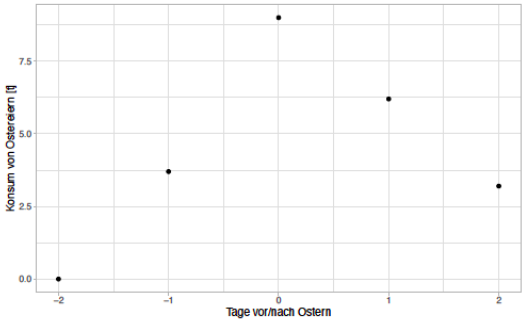


Figure 5: Graph for task 5

| | Männer | Frauen |
|---|---|---|
| Hund | 191 | 206 |
| Katze | 257 | 312 |
| Beides | 58 | 69 |
| Keins von beiden | 1254 | 1120 |

Figure 6: Graph for task 6

c) *For non-Media Informatics students* Calculate and interpret the contingency coefficient $K$ and the corrected coefficient $K^*$. What is the main difference between them? (*calculation; correlation*)

d) *For Media Informatics students* Given a $3 \times 4$ contingency table, write R code to transform $K$ into $K^*$. (*calculation; correlation*)

## Task 7

A dataset of 10 households provides monthly income $X$ and summer vacation expenses $Y$.

a) Interpret the meaning of the estimated slope coefficient $\hat{\beta}_1$ in the context. (*interpretation; regression*)

b) Calculate the intercept $\hat{\beta}_0$ using the given value $\bar{y} = 1179.3$. (*calculation; regression*)

c) Predict vacation expenses for a monthly income of 2000 EUR. If you were not able to calculate $\hat{\beta}_0$ in the previous task, use $\hat{\beta}_0 = 160$. (*calculation; regression*)

d) Given $R^2 = 0.95$, what does this say about the strength of the relationship between $X$ and $Y$? Can you determine the exact Spearman rank correlation coefficient? (*interpretation; regression*)

| $i$ | 1 | 2 | 3 | 4 | 5 | 6 | 7 | 8 | 9 | 10 |
|---|---|---|---|---|---|---|---|---|---|---|
| $y_i$ | 1296 | 796 | 1753 | 1344 | 569 | 1257 | 636 | 1546 | 1132 | 1464 |
| $x_i$ | 3413 | 2276 | 5374 | 4410 | 1413 | 3862 | 1764 | 4550 | 3022 | 3868 |

Figure 7: Graph for task 7

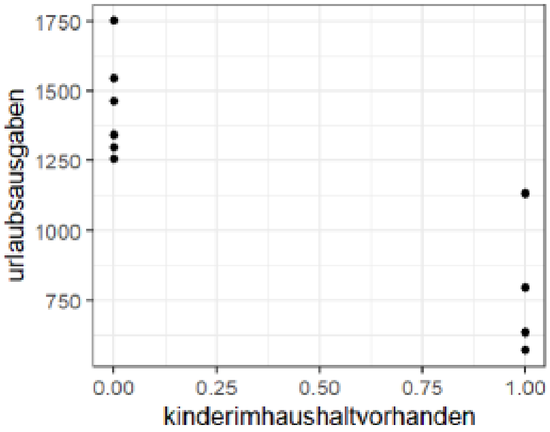


Figure 8: Graph for task 7f

```
Call:
lm(formula = urlaubsausgaben ~ monatseinkommen + kinderimhaushaltvorhanden)

Residuals:
    Min      1Q  Median      3Q     Max 
-145.03  -44.01  -11.15   68.27  126.14 

Coefficients:
                           Estimate Std. Error t value Pr(>|t|)    
(Intercept)               259.02195  210.44993   1.231 0.258145    
monatseinkommen             0.27891    0.04871   5.727 0.000715 ***
kinderimhaushaltvorhanden -66.71902  120.55025  -0.553 0.597178    
---
Signif. codes:  0 '***' 0.001 '**' 0.01 '*' 0.05 '.' 0.1 ' ' 1

Residual standard error: 95.45 on 7 degrees of freedom
Multiple R-squared:  0.9547,    Adjusted R-squared:  0.9418 
F-statistic: 73.79 on 2 and 7 DF,  p-value: 1.976e-05
```

Figure 9: Graph for task 7g

e) Would you use the model to predict vacation expenses for very low incomes (<500 EUR)? Why or why not? (*interpretation; regression*)

f) A new variable "children in household" (1 = yes, 0 = no) is added. Is it possible to regress vacation expenses on this variable? Would you expect the coefficient to be positive or negative based on the scatterplot? (*interpretation; regression*)

g) Interpret the coefficients from a multiple regression with vacation expenses as dependent variable and "children in household" plus monthly income as independent variables. Use the given R output. (*interpretation; regression*)

h) Predict vacation expenses for a household with two children and monthly income of 2700 EUR. (*interpretation; regression*)
